# Supplementary material for: SocialGesture: Delving into Multi-person Gesture Understanding
Source: arXiv:2504.02244 source file (2025-04-03)
Supplement: Supplementary file 1 [file appendix.tex]

\clearpage
\setcounter{page}{1}
% \maketitlesupplementary

\section{Dataset}
\label{sec:appendix_dataset}
